# Supplementary material for: Atomistic Mechanisms of Sliding in Few-Layer and Bulk Doped MoS$_2$
Source: arXiv:2209.15629 ancillary file (2022-09-30)
Supplement: Supplementary file 1 [file SI.pdf]

# Supporting Information: Atomistic Mechanisms of Sliding in Few-Layer and Bulk Doped $MoS_2$

Enrique Guerrero[†*] and David A. Strubbe[†*]

[†] *Department of Physics, University of California, Merced, Merced, CA 95343*

E-mail: eguerrero23@ucmerced.edu; dstrubbe@ucmerced.edu

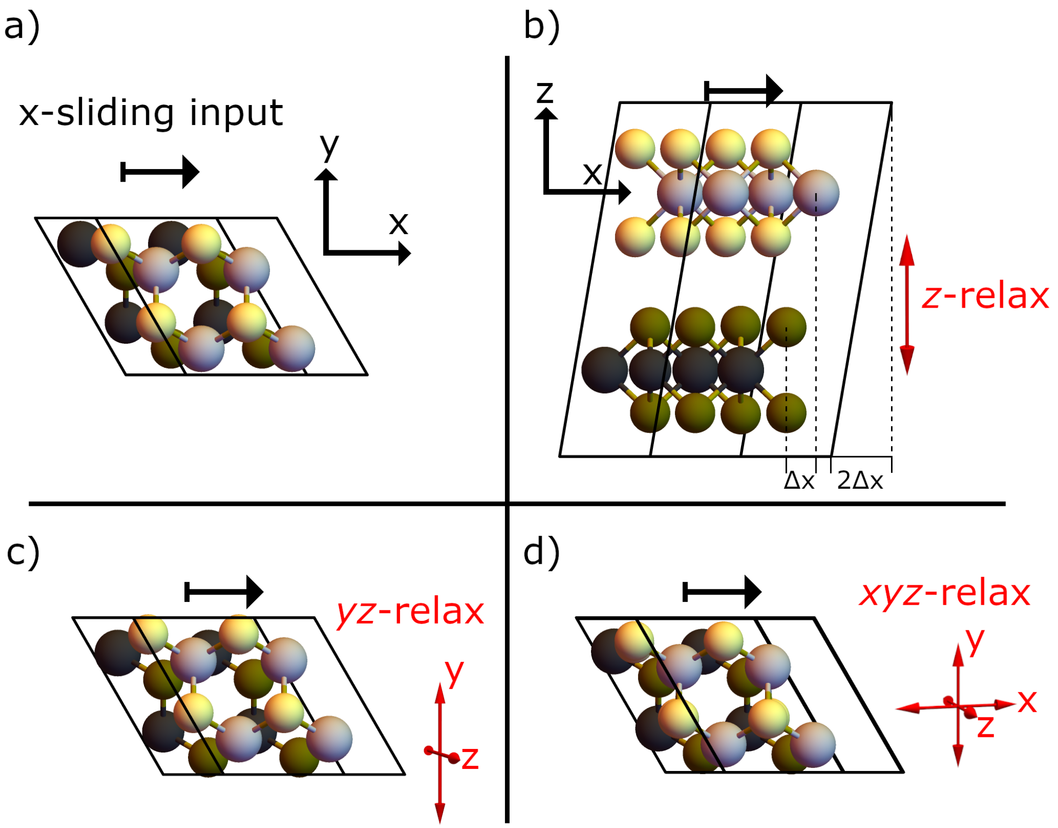


Figure S1: $x$-sliding was analyzed using four kinds of calculations, with relaxation of an increasing number of degrees of freedom of the Mo and S atoms. a) No relaxation, b) $z$-relax, c) $yz$-relax and d) $xyz$-relax. Dark atoms indicate the lower layer. The Ni atom's coordinates are fully relaxed in b)-d).

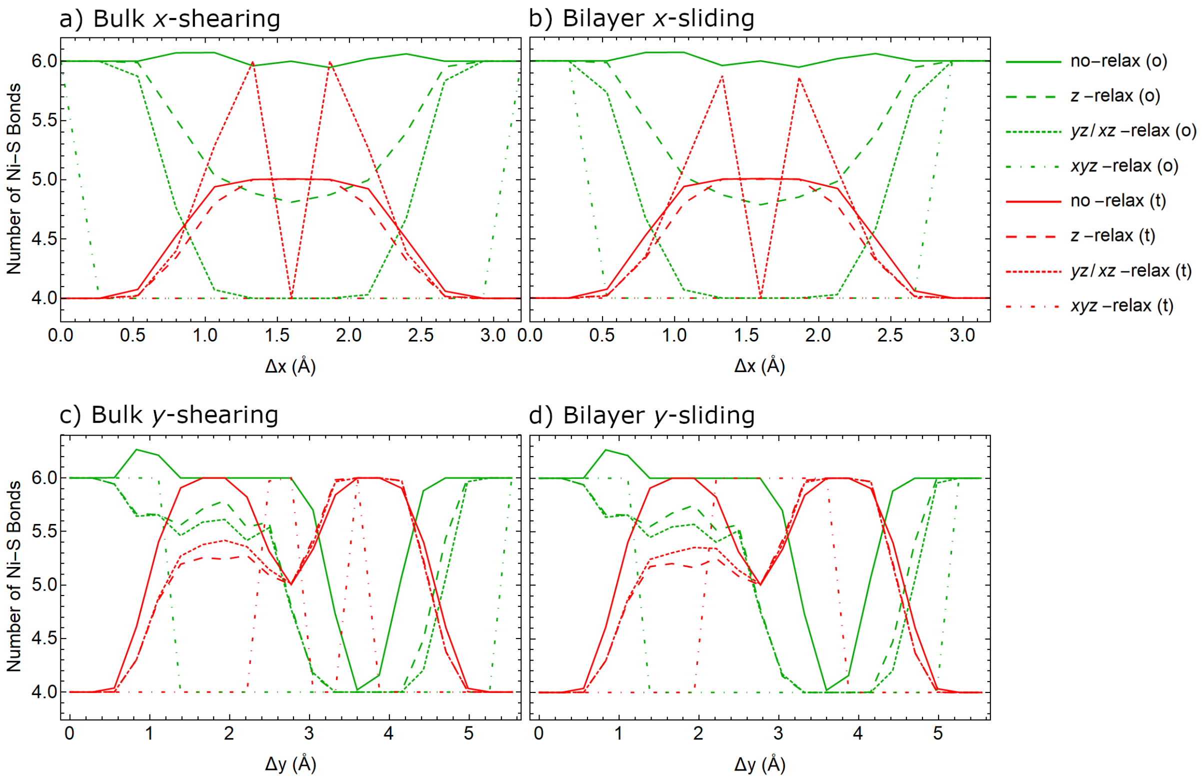


Figure S2: Bond count as a function of sliding for o-intercalated (green) and t-intercalated (red) structures at the four constraint levels as computed by the Tersoff bond order function for a) $x$-shearing in bulk, b) $x$-sliding in bilayers, c) $y$-shearing in bulk, and d) $y$-sliding in bilayers. Having the most freedom, $xyz$-relaxed structures reorganize to form four bonds, even at less favorable stacking. The large spike at $\Delta x = 1.6$ Å for t-intercalated $yz$-relax is the result of the structure reorganizing to a stacking equivalent to the $\Delta x = 0$ Å configuration. a) and b) are nearly identical.

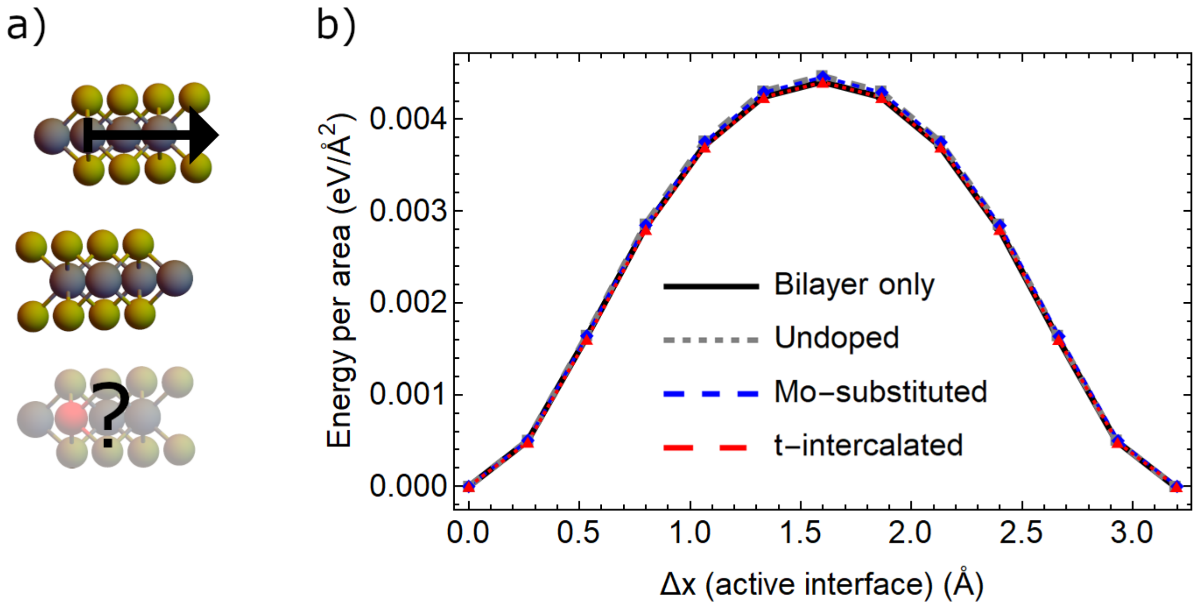


Figure S3: Sliding in three-layer systems *vs.* undoped bilayer (black). The top pair of layers are undoped and are slid next to each other then relaxed in the $z$-direction. The sliding energy is divided by the area of the active sliding area, so as to keep it comparable with the bilayer. The presence of a third layer (doped or undoped) does not change the sliding potential by more than 1.5%.

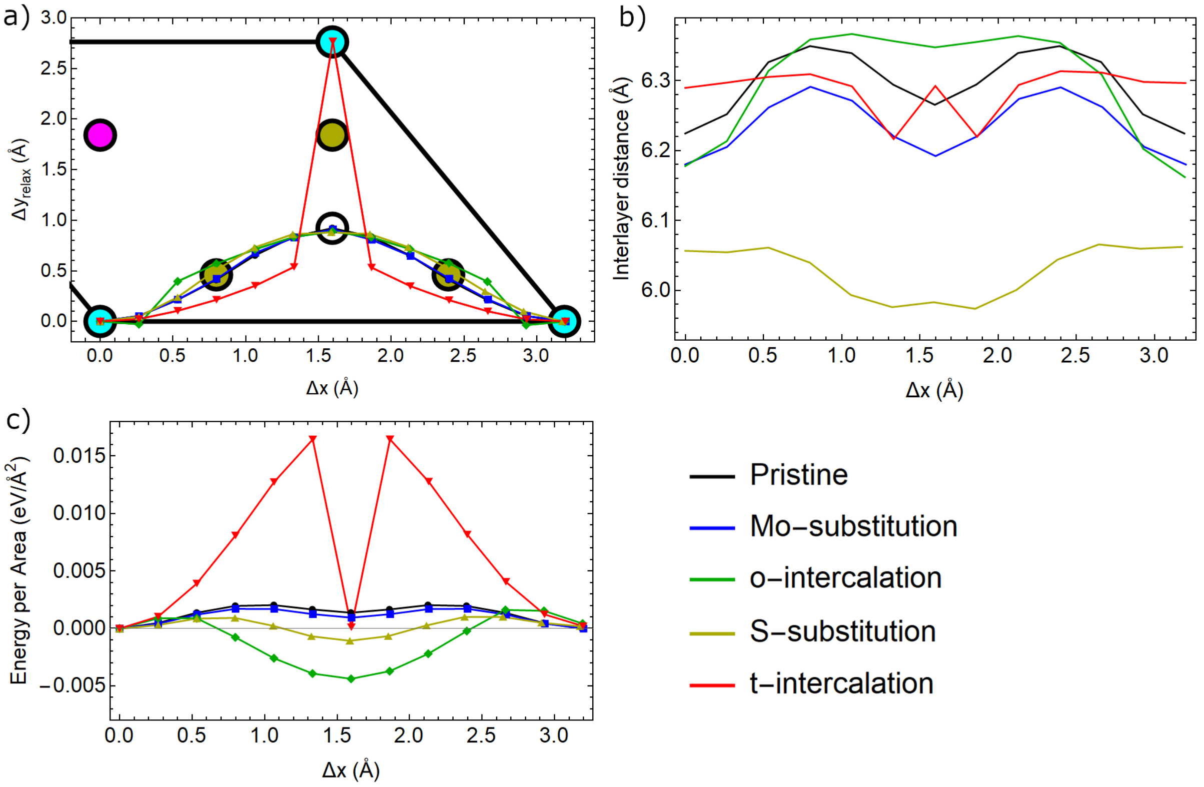


Figure S4: a) Sliding path under $yz$-relax constraints of bilayers slid in the $x$-direction. Deviations from the pristine zigzag path are slightly more pronounced in all cases. Colored circles mark high-symmetry stacking and extrema for S substitution, as in Fig. 3. b) Interlayer distances show identical pattern to bulk shearing, albeit at a slightly larger value as compared in Fig. S5. c) Sliding energies divided by one cell's area.

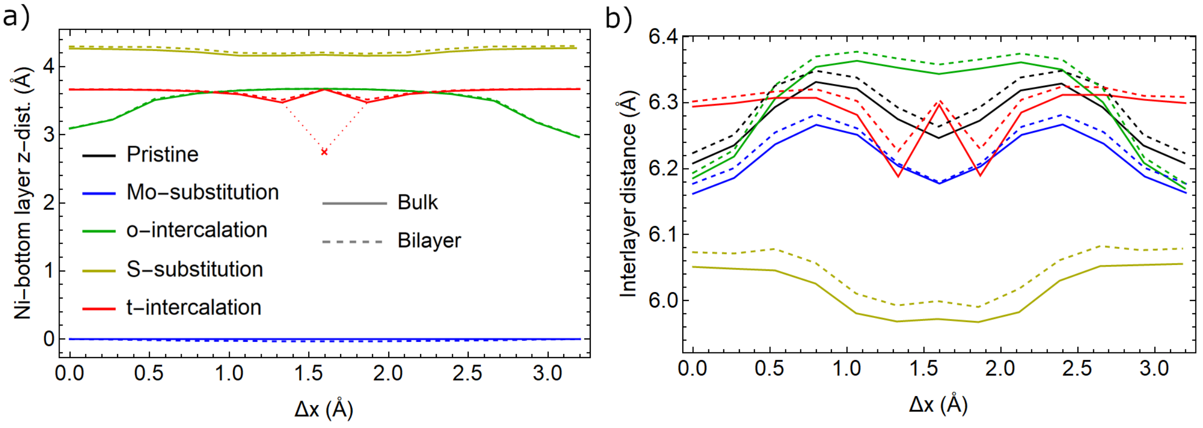


Figure S5: a) Ni $z$-coordinate with respect to the bottom layer (see Fig. 1 for relative Ni positions) under $xz$-relax. The red × indicates the t-intercalated structure that used a different generation scheme to relax it near the AB′ stacking configuration. b) Mo-Mo interlayer distances comparing bilayer (dashed) to bulk (solid) for $xz$-relax.

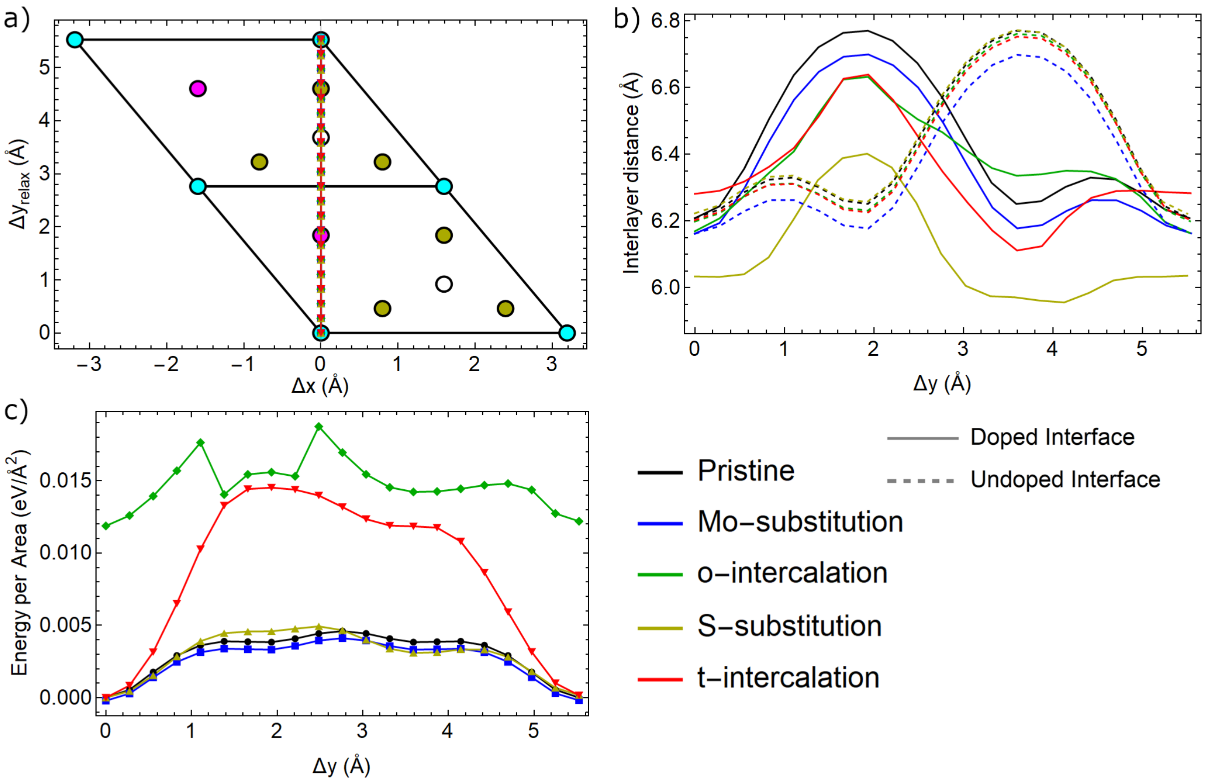


Figure S6: Relative sliding for $y$-sliding of bulk and bilayer with $xz$-relax constraints. a) Sliding path with respect to the pristine cell sites. Cyan, white, and magenta circles indicate AA′, $AB_1$, and $AB_2$, respectively. Yellow circles represent locations of energy extrema for S substitution. Unlike in $x$-sliding, the structure did not deviate much ($\sim 10^{-4}$ Å) from the path, despite being given freedom in the $x$-coordinates. b) Interlayer distances. The Mo-Mo interlayer distance shows little difference between sites in the undoped interfaces, but the doped interfaces vary in shape with S-substitution and intercalations showing greatest variabilities. c) Sliding energies (divided by twice the cell's area, once for each active sliding interface), which lack the mirror-symmetry seen in $x$-sliding. Ni in the o-intercalation case switches to t-intercalation around $1.5 - 2.0$ Å. Both intercalated energies are referenced to the $\Delta y = 0$ Åt-intercalated structure.

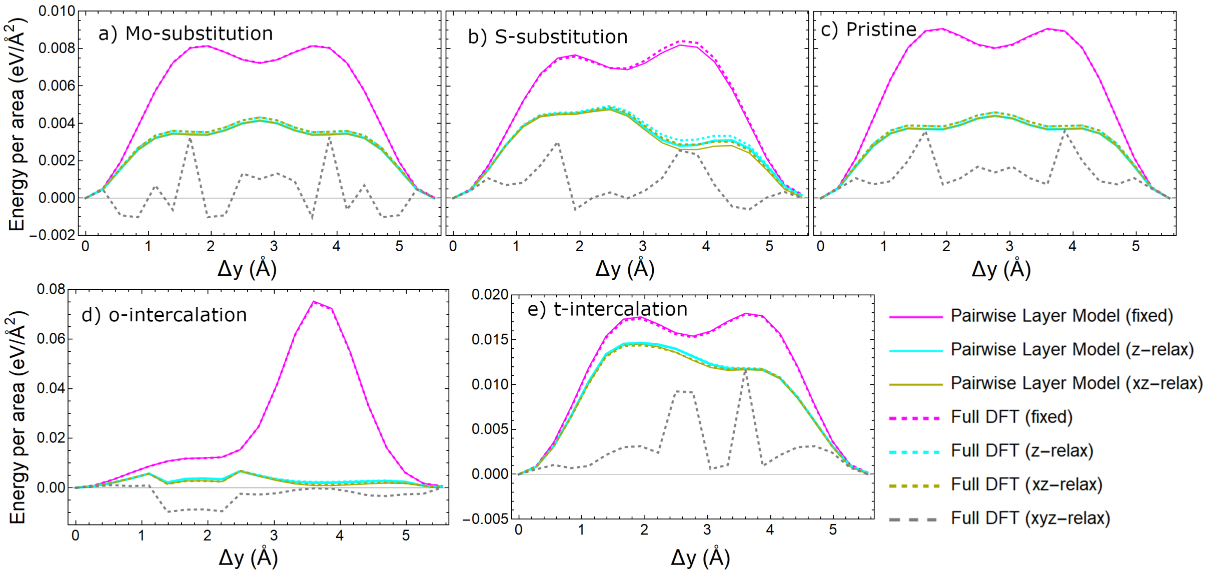


Figure S7: Energies per sliding-active layer are plotted for the different doped structures. Full bulk DFT (solid) and pairwise combinations of bilayers (dashed) for doped $MoS_2$. The $y$-direction sliding potential for a single pristine interface is not symmetric, but the two interfaces in the bulk 2H structure are sliding in opposite orientations. This leads to a 180° rotation symmetry in c) pristine, which is broken in the doped structures. Bulk sliding potentials for b) S-substitution, d) o-intercalation, and e) t-intercalation are computed as sums of the doped bilayer and the undoped potential. Bulk a) Mo-substitution and c) pristine potentials are sums of the corresponding bilayer potential and this potential reflected across the midpoint, to account for the opposite interlayer sliding orientations.

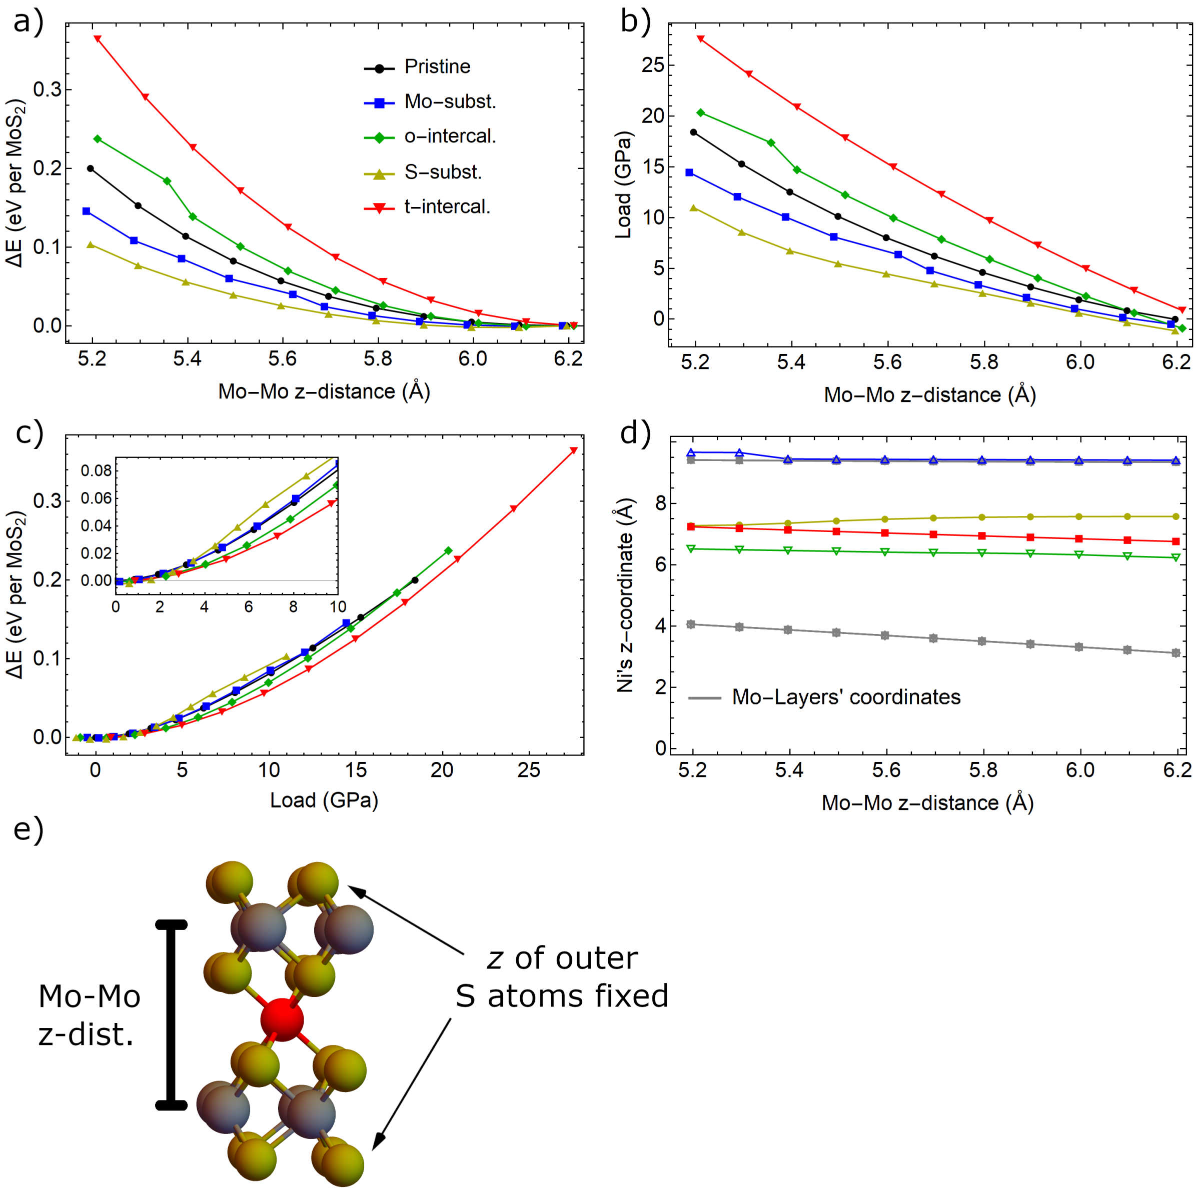


Figure S8: Computations of load applied to the bilayer of $2 \times 2$ supercells, without sliding. The layers are compressed and the $z$-coordinates of the outer S atoms are fixed, as shown in e). All other atomic coordinates and the cell parameters $a$ and $b$ are allowed to relax. The relative energy a) and load b), computed as the sum of the forces on the upper fixed S-atoms divided by the cross-sectional area, are plotted against the Mo-Mo $z$-separation, or interlayer distance. Loads show an ordering similar to the elastic moduli $C_{33}$ we previously computed,[S1] except for S substitution. Energies and loads of intercalated $MoS_2$ are more sensitive to compression than pristine $MoS_2$, opposite to the substituted structures. Load *vs.* $\Delta E$ c) and inset show behavior for S substitution which is not just a rescaling of the pristine trend. d) Ni $z$-coordinates for the different doped structures are plotted along with the layers' coordinates (gray). Ni substituting for S is attracted to the opposite layer with increased compression, whereas Ni moves away along with the closer layer in t-intercalation. This explains the different behavior of S-substitution in b) and c).

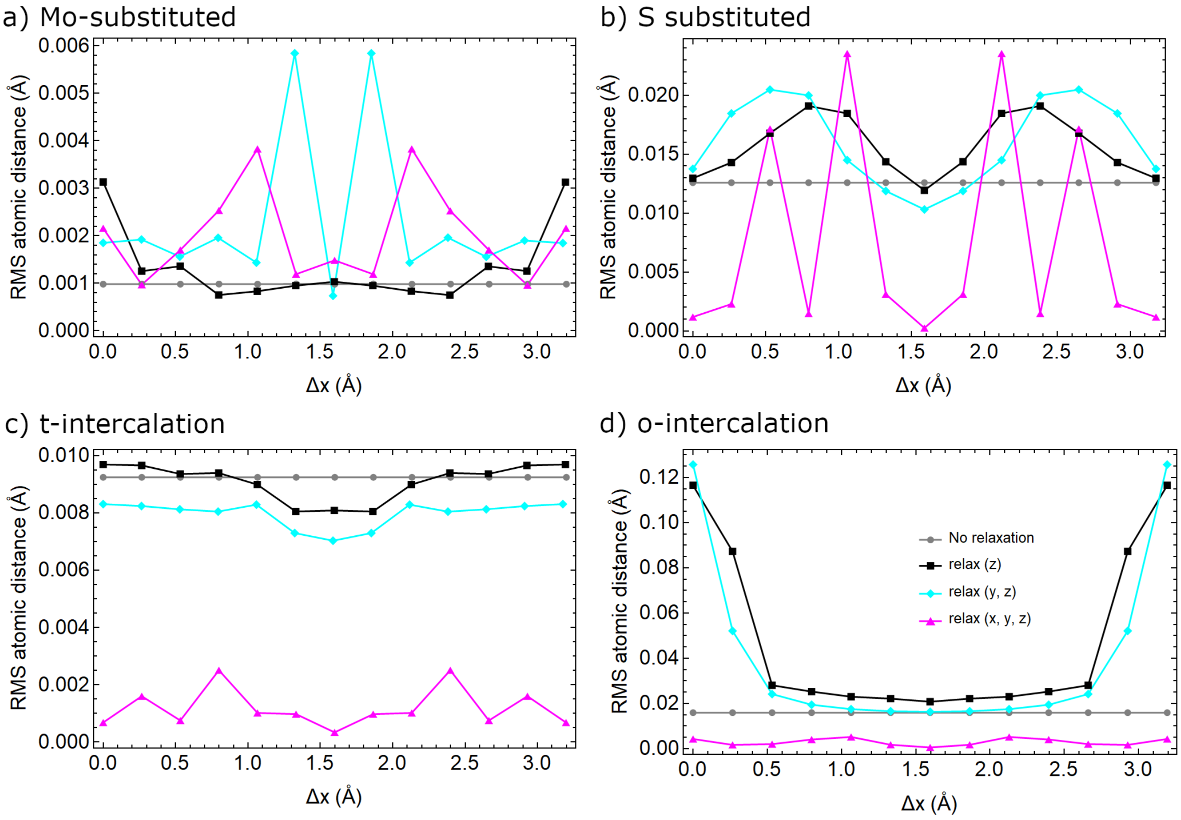


Figure S9: Deviations from symmetry in sliding, expressed by root mean square (RMS) differences of the atomic coordinates between a bulk structure slid by identical displacements in the positive and negative $x$ directions. These are computed by taking the structure slid by $\Delta x$, reflecting across the $yz$-plane ($\sigma_{yz}$), then comparing to its nearly symmetric counterpart, at $a_p - \Delta x$, where $a_p$ is the pristine lattice constant. Coordinates are compared between closest corresponding atoms.

$$\mathrm{RMS} = \sqrt{\sum_i \left|\sigma_{yz}\mathbf{R}_i(\Delta x) - \mathbf{R}_i(a_p - \Delta x)\right|^2}$$

## References

(S1) Guerrero, E.; Karkee, R.; Strubbe, D. A. Phase Stability and Raman/IR Signatures of Ni-doped $MoS_2$ from Density Functional Theory Studies. *J. Phys. Chem. C* **2021**, *125*, 13401–13412.
